# Supplementary material for: Bridging Modalities and Transferring Knowledge: Enhanced Multimodal Understanding and Recognition
Source: arXiv:2512.20501 source file (2025-12-23)
Supplement: Supplementary file 1 [file bmvc2021_appendix.tex]

\chapter{Appendix for Multimodal Fusion for Improving Compositional Action Recognition}\label{bmvc2021:appendix:ch:bmvc2021:appendix}
The Supplementary material is organized as follows:

\begin{itemize}
    \item Details on the appearance (RGB-based) models (\S\ref{bmvc2021:appendix:sec:appearance}).
    % \item Details on the multimodal fusion approaches (\S\ref{bmvc2021:appendix:sec:fusion}).
    \item Details on the object detections-based methods (\S\ref{bmvc2021:appendix:sec:layout}).
    \item Implementation details (\S\ref{bmvc2021:appendix:sec:experimental-setup}).
    % \item Details about the datasets (\S\ref{bmvc2021:appendix:sec:datasets}).
    \item Details the object detector we train on Action Genome (\S\ref{bmvc2021:appendix:sec:genome-object-detector}).
    \item Additional qualitative evaluation (\S\ref{bmvc2021:appendix:sec:qualitative}).
\end{itemize}

\section{Appearance Models}\label{bmvc2021:appendix:sec:appearance}
% In \S\ref{bmvc2021:sec:appearance-fusion}, we discuss the different appearance models we make use of, as well as the multimodal fusion methods employed to combine the appearance and layout (STLT) features.
As an appearance model, we deem a neural network, typically a convolutional neural network (CNN), that takes as input a sequence of video frames $v_1, v_2, ..., v_T$, where $T$ is the number of video frames we sample from the video. In certain cases, i.e., with EF, CAF, and CACNF we sample a different number of appearance- and layout-based frames.
% Each $v_i \in \mathbb{R}^{C \times H \times W}$, where $C$ is the number of channels (in our case $C = 3$, as we deal with RGB frames), and $H$ and $W$ are the video height and width, while $V \in \mathbb{R}^{C \times T \times H \times W}$.
Depending on the corresponding appearance model, we sample a different set of video frames, as well as pre-process these frames differently during training and evaluation.

\subsubsection{2D Resnet152}\label{bmvc2021:appendix:sec:2d-resnet152}
With the 2D Resnet152 \cite{he2016deep} (abbreviated as R2D-152), for each sampled spatial layout frame we sample its corresponding RGB frame, i.e., the frame from where we take the spatial layout (bounding boxes and object categories). As the R2D-152 model was pre-trained on ImageNet \cite{deng2009imagenet}, we follow the ImageNet way of pre-processing. To be specific, we firstly rescale each frame so that its shorter side length is 256, and then take a center crop of size 224 $\times$ 224. Each video frame is subsequently per-channel normalized as per standard practice \cite{he2016deep}. We take the output of the R2D-152's penultimate layer, i.e., the layer before the classifier, yielding a frame embedding of size 2048. We concatenate the embeddings of each frame to form a sequence, yielding a video appearance embedding $\mathbf{\hat{A}} \in \mathbb{R}^{T \times 2048}$.

\subsubsection{2D Resnet50 backbone from Faster R-CNN}\label{bmvc2021:appendix:sec:resnet50-backbone}
We extract the Resnet50 backbone from a Faster R-CNN \cite{ren2015faster} trained on the task of COCO \cite{lin2014microsoft} object detection. We abbreviate this model as R2D-50. With the R2D-50 appearance model, to obtain video appearance information, besides the video frames themselves, we additionally utilize the bounding boxes, i.e., the spatial layouts. Given a video frame and its object detections, we firstly pre-process the video frame with the standard Faster R-CNN pre-processing \cite{ren2015faster}, and obtain RoI Align \cite{he2017mask} features from each region of interest (as defined by the object detections). Each region of interest feature is of size $256 \times 7 \times 7$, which we average-pool to $256 \times 3 \times 3$, and then flatten to a vector of size 2304.

\subsubsection{3D Resnet50}\label{bmvc2021:appendix:sec:r3d-appendix}
While the input to R2D-152 and R2D-50 is individual frames, with no temporal connectivity between them, with the 3D Resnet50 (abbreviated as R3D or R3D-50), we exploit the temporal connectivity of the frames. To that end, we use a 3D Resnet50 \cite{kataoka2020would}, pre-trained on Kinetics-700 \cite{carreira2019short}, Moments in Time \cite{monfort2019moments} and Stair Actions \cite{yoshikawa2018stair}. The input to R3D is a frame sequence $v_1, v_2, ..., v_T$. During training, we sample a random contiguous sequence of frames, while during evaluation, we sample a contiguous sequence of frames from the center of the video. Note that the sampling of frames is identical to \cite{materzynska2020something} for accurate state-of-the-art comparisons (\S\ref{bmvc2021:sec:state-of-the-art}). We first rescale each frame so that the shorter side is of size 128. Then, during training, we take a random crop of 112 $\times$ 112 across all frames, and during inference, we take a center crop of 112 $\times$ 112 across all frames (see \S\ref{bmvc2021:appendix:sec:experimental-setup} for more details). Finally, we forward-propagate the pre-processed video frames through R3D, yielding a video embedding $\mathbf{\hat{A}} \in \mathbb{R}^{2048 \times T_d \times H_d \times W_d}$, where $_d$ indicates downscaled, and 2048 is the R3D penultimate layer hidden size.

\subsubsection{3D-Resnet50 Transformer}
With the 3D-Resnet50 Transformer appearance model (R3D-Transformer), we reuse R3D, as defined and explained in \S~\ref{bmvc2021:appendix:sec:r3d-appendix}, and we add a transformer model \cite{vaswani2017attention} on top. Namely, given the output video embedding from R3D, we firstly use an additional $\operatorname{Conv3D}$ layer with a kernel size $1 \times 1 \times 1$ to project it in the desired hidden dimensionality $\mathbf{\hat{A}} \in \mathbb{R}^{Z \times T_d \times H_d \times W_d}$, where $Z$ is the hidden size. We flatten the embedding across the temporal and spatial dimension $\mathbb{R}^{Z \times T_d * H_d * W_d}$, essentially making it a sequence, and append a special \texttt{class} embedding. We sum the R3D embedding with additional positional embeddings to inject positional information. We forward-propagate the obtained embeddings through the transformer, yielding a sequence of hidden states as output.

\section{Baseline Object Detections-based Models}\label{bmvc2021:appendix:sec:layout}
In \S\ref{bmvc2021:sec:eval}, we compare \blackgls{stlt} performance on the Something-Else compositional dataset and the Something-Something V2 dataset against
\begin{inparaenum}[(i)]
\item GNN-NL: A baseline model \cite{materzynska2020something} utilizing a graph neural network \cite{kipf2017semi} for spatial reasoning and a non-local neural network \cite{wang2018non} for temporal reasoning. Essentially, our implementation of STIN \cite{materzynska2020something}, where we train the model within our setup (optimizer, learning rate scheduler, training epochs, etc.). Refer to \cite{materzynska2020something} for details;
\item S\&TLT: An \blackgls{stlt} variant, where the spatial and temporal reasoning are performed jointly.
\end{inparaenum}

\subsection{Spatial \& Temporal Layout Transformer}
With the Spatial \& Temporal Layout Transformer, abbreviated as \blackgls{s_and_tlt}, instead of having decoupled spatial and temporal reasoning over the spatio-temporal layouts, we perform it jointly. Similar to \blackgls{stlt}, we obtain the category embedding $\mathbf{\hat{c}}_j$ and the location in the frame embedding $\mathbf{\hat{l}}_j$ with two separate fully-connected layers. However, in this case, for each frame object $o_j$, we additionally obtain its frame position index, where 
%, e.g., if the object is from the first frame the index would be $0$, while if it is from the last frame, it would be $n$, where
$n$ is the number of sampled video frames.
Therefore, for a single object, we obtain its embedding as $\mathbf{\hat{o}}_j = \operatorname{Dropout}(\operatorname{LayerNorm}(\mathbf{\hat{c}}_j + \mathbf{\hat{l}}_j + \mathbf{\hat{p}}_j))$, where an additional fully-connected layer yields the $\mathbf{\hat{p}}_j$ embedding. Finally, we append a special \texttt{class} object embedding $\mathbf{\hat{o}}_{\text{\texttt{class}}}$ at the sequence end, and forward-propagate the sequence of object embeddings through a transformer model. We control the attention pattern using an attention mask, such that for objects spanning a single frame we perform bidirectional attention, while we perform causal attention across the video.

\section{Implementation Details}\label{bmvc2021:appendix:sec:experimental-setup}
For all layout-based models, we randomly sample 16 frames represented as spatio-temporal layouts. For models using an R3D appearance model, we uniformly sample 32 frames from the video, and then resize the frames so that the size of the smaller side is 128. During training, we randomly crop the frames to 112 $\times$ 112 and apply color jittering. During inference, we take a center crop of size 112 $\times$ 112.

We train all models for 20 epochs with AdamW \cite{loshchilov2018decoupled}, with a peak learning rate of $5e-5$, linearly warmed-up for the first 10\% of the training, and decreased to $0.0$ until the end. We apply weight decay of $1e-3$, gradient clipping when the norm exceeds $5.0$, and dropout \cite{srivastava2014dropout} of $0.1$ in the attention and feed-forward modules (the bias term, the positional and \texttt{class} embeddings are excluded from the weight decay).
We use 4 and 8 multi-head self-attention layers for the spatial and temporal transformer in \blackgls{stlt} respectively, and 4 cross- and self-attention in \blackgls{caf} and \blackgls{cacnf}. The hidden size for all modules is 768.

On the Something-Something and Something-Else dataset, only two object categories are registered in STLT---``hand'' or ``object''. On the Action Genome dataset, we register all 36 object categories present in the dataset (also predicted by the trained object detector)---``hair'', ``book'', ``medicine'', ``vacuum'', ``food'', ``groceries'', ``floor'', ``mirror'', ``cabinet'', ``doorway'', ``notebook'', ``picture'', ``phone'', ``couch'', ``sandwich'', ``bottle'', ``towel'', ``box'', ``blanket'', ``television'', ``bag'', ``refrigerator'', ``table'', ``light'', ``broom'', ``shoe'', ``doorknob'', ``bed'', ``window'', ``shelf'', ``door'', ``pillow'', ``laptop'', ``dish'', ``clothes'' and ``person''.

All models trained on the Something-Something and the Something-Else datasets minimize the cross-entropy loss, while all models trained on the Action Genome dataset minimize the per-class binary cross-entropy loss during training.

\section{Action Genome: Object Detector Training}\label{bmvc2021:appendix:sec:genome-object-detector}
The Action Genome dataset \cite{ji2020action}, built on top of Charades \cite{sigurdsson2016hollywood}, provides bounding box and object category annotations for a random subset of frames where the action occurs in each video. Besides utilizing these in the ``oracle'' experiments, we train a Faster R-CNN \cite{ren2015faster} object detector to create an ``object predictions'' (obj. predictions) setting. For training the object detector we use the standard train/validation Charades split. Using Detectron2 \cite{wu2019detectron2}, we train a Faster R-CNN with a Resnet101 \cite{he2016deep} backbone, which was pre-trained on the COCO \cite{lin2014microsoft} dataset. We train the model with stochastic gradient descent (SGD) for 5 epochs, with a learning rate of $1e-5$. During training, we apply random horizontal flipping of the frames. We obtain an average precision (AP) of 11.3 on the Action Genome validation set. When generating the spatio-temporal layouts, we keep all object detections with a probability of at least 0.5.

\section{Additional Qualitative Evaluation}\label{bmvc2021:appendix:sec:qualitative}
\begin{figure*}[t]
\centering
\includegraphics[width=1.0\textwidth]{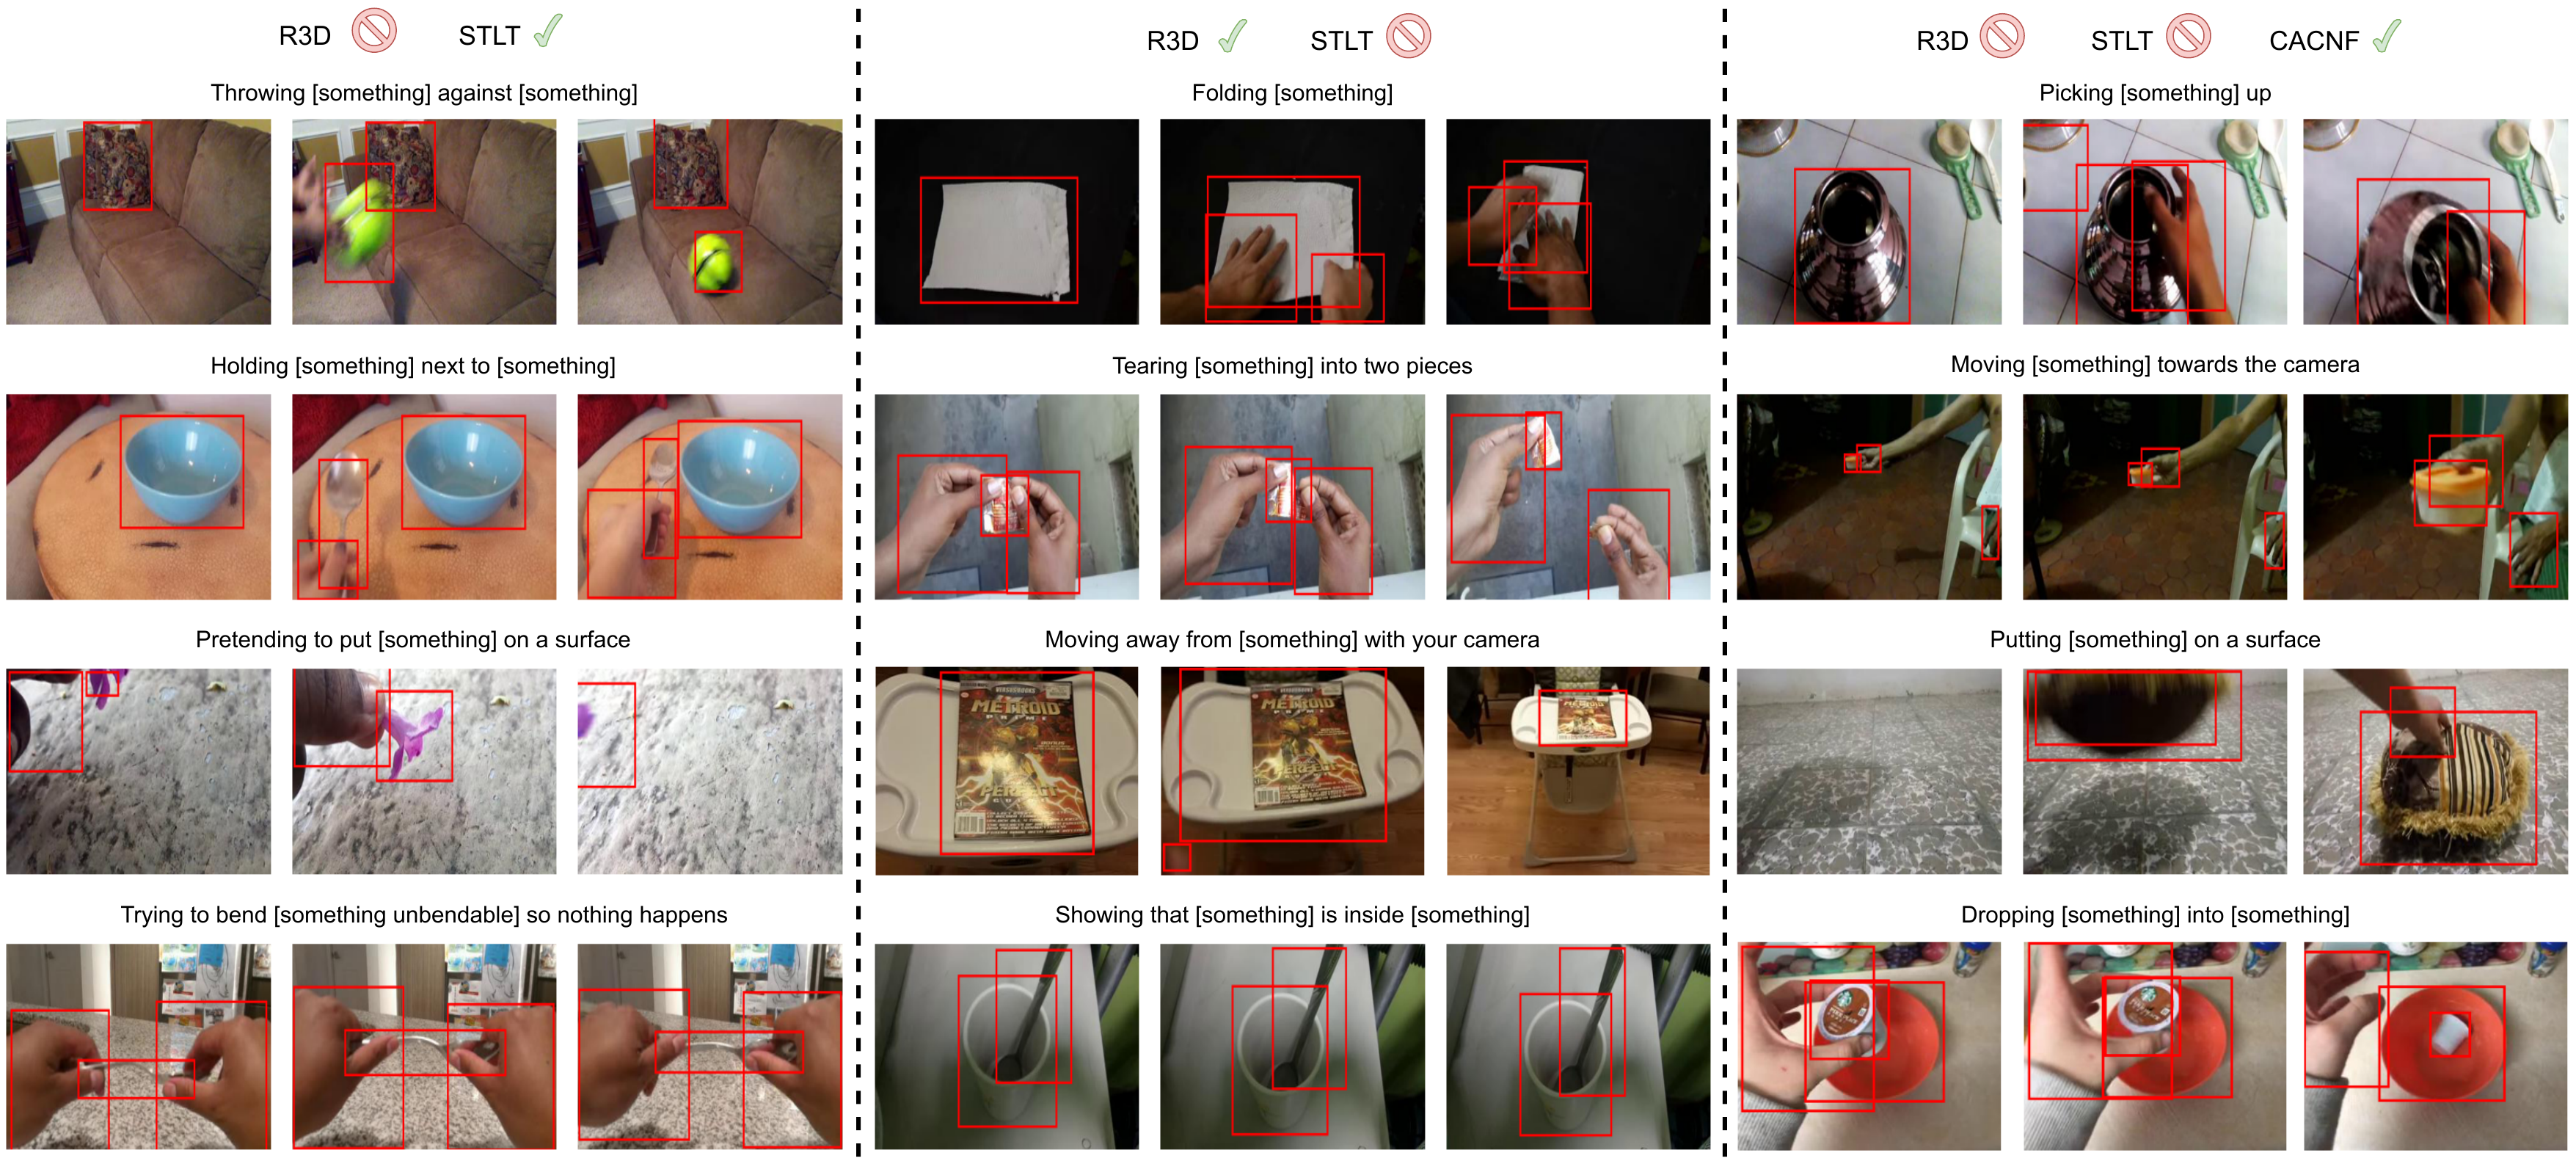}
\caption[Qualitative evaluation on the Something-Else compositional dataset.]{Qualitative evaluation on the Something-Else compositional dataset. \textbf{Left:} R3D mispredicts, STLT predicts correctly. \textbf{Middle:} STLT mispredicts, R3D predicts correctly. \textbf{Right:} \blackgls{stlt} and R3D mispredict, \blackgls{cacnf} predicts correctly. Above each set of video frames is the ground truth action class.}
\label{bmvc2021:appendix:fig:qualitative-smth-appendix}
\end{figure*}

\begin{figure*}[!ht]
\centering
\includegraphics[width=0.95\textwidth]{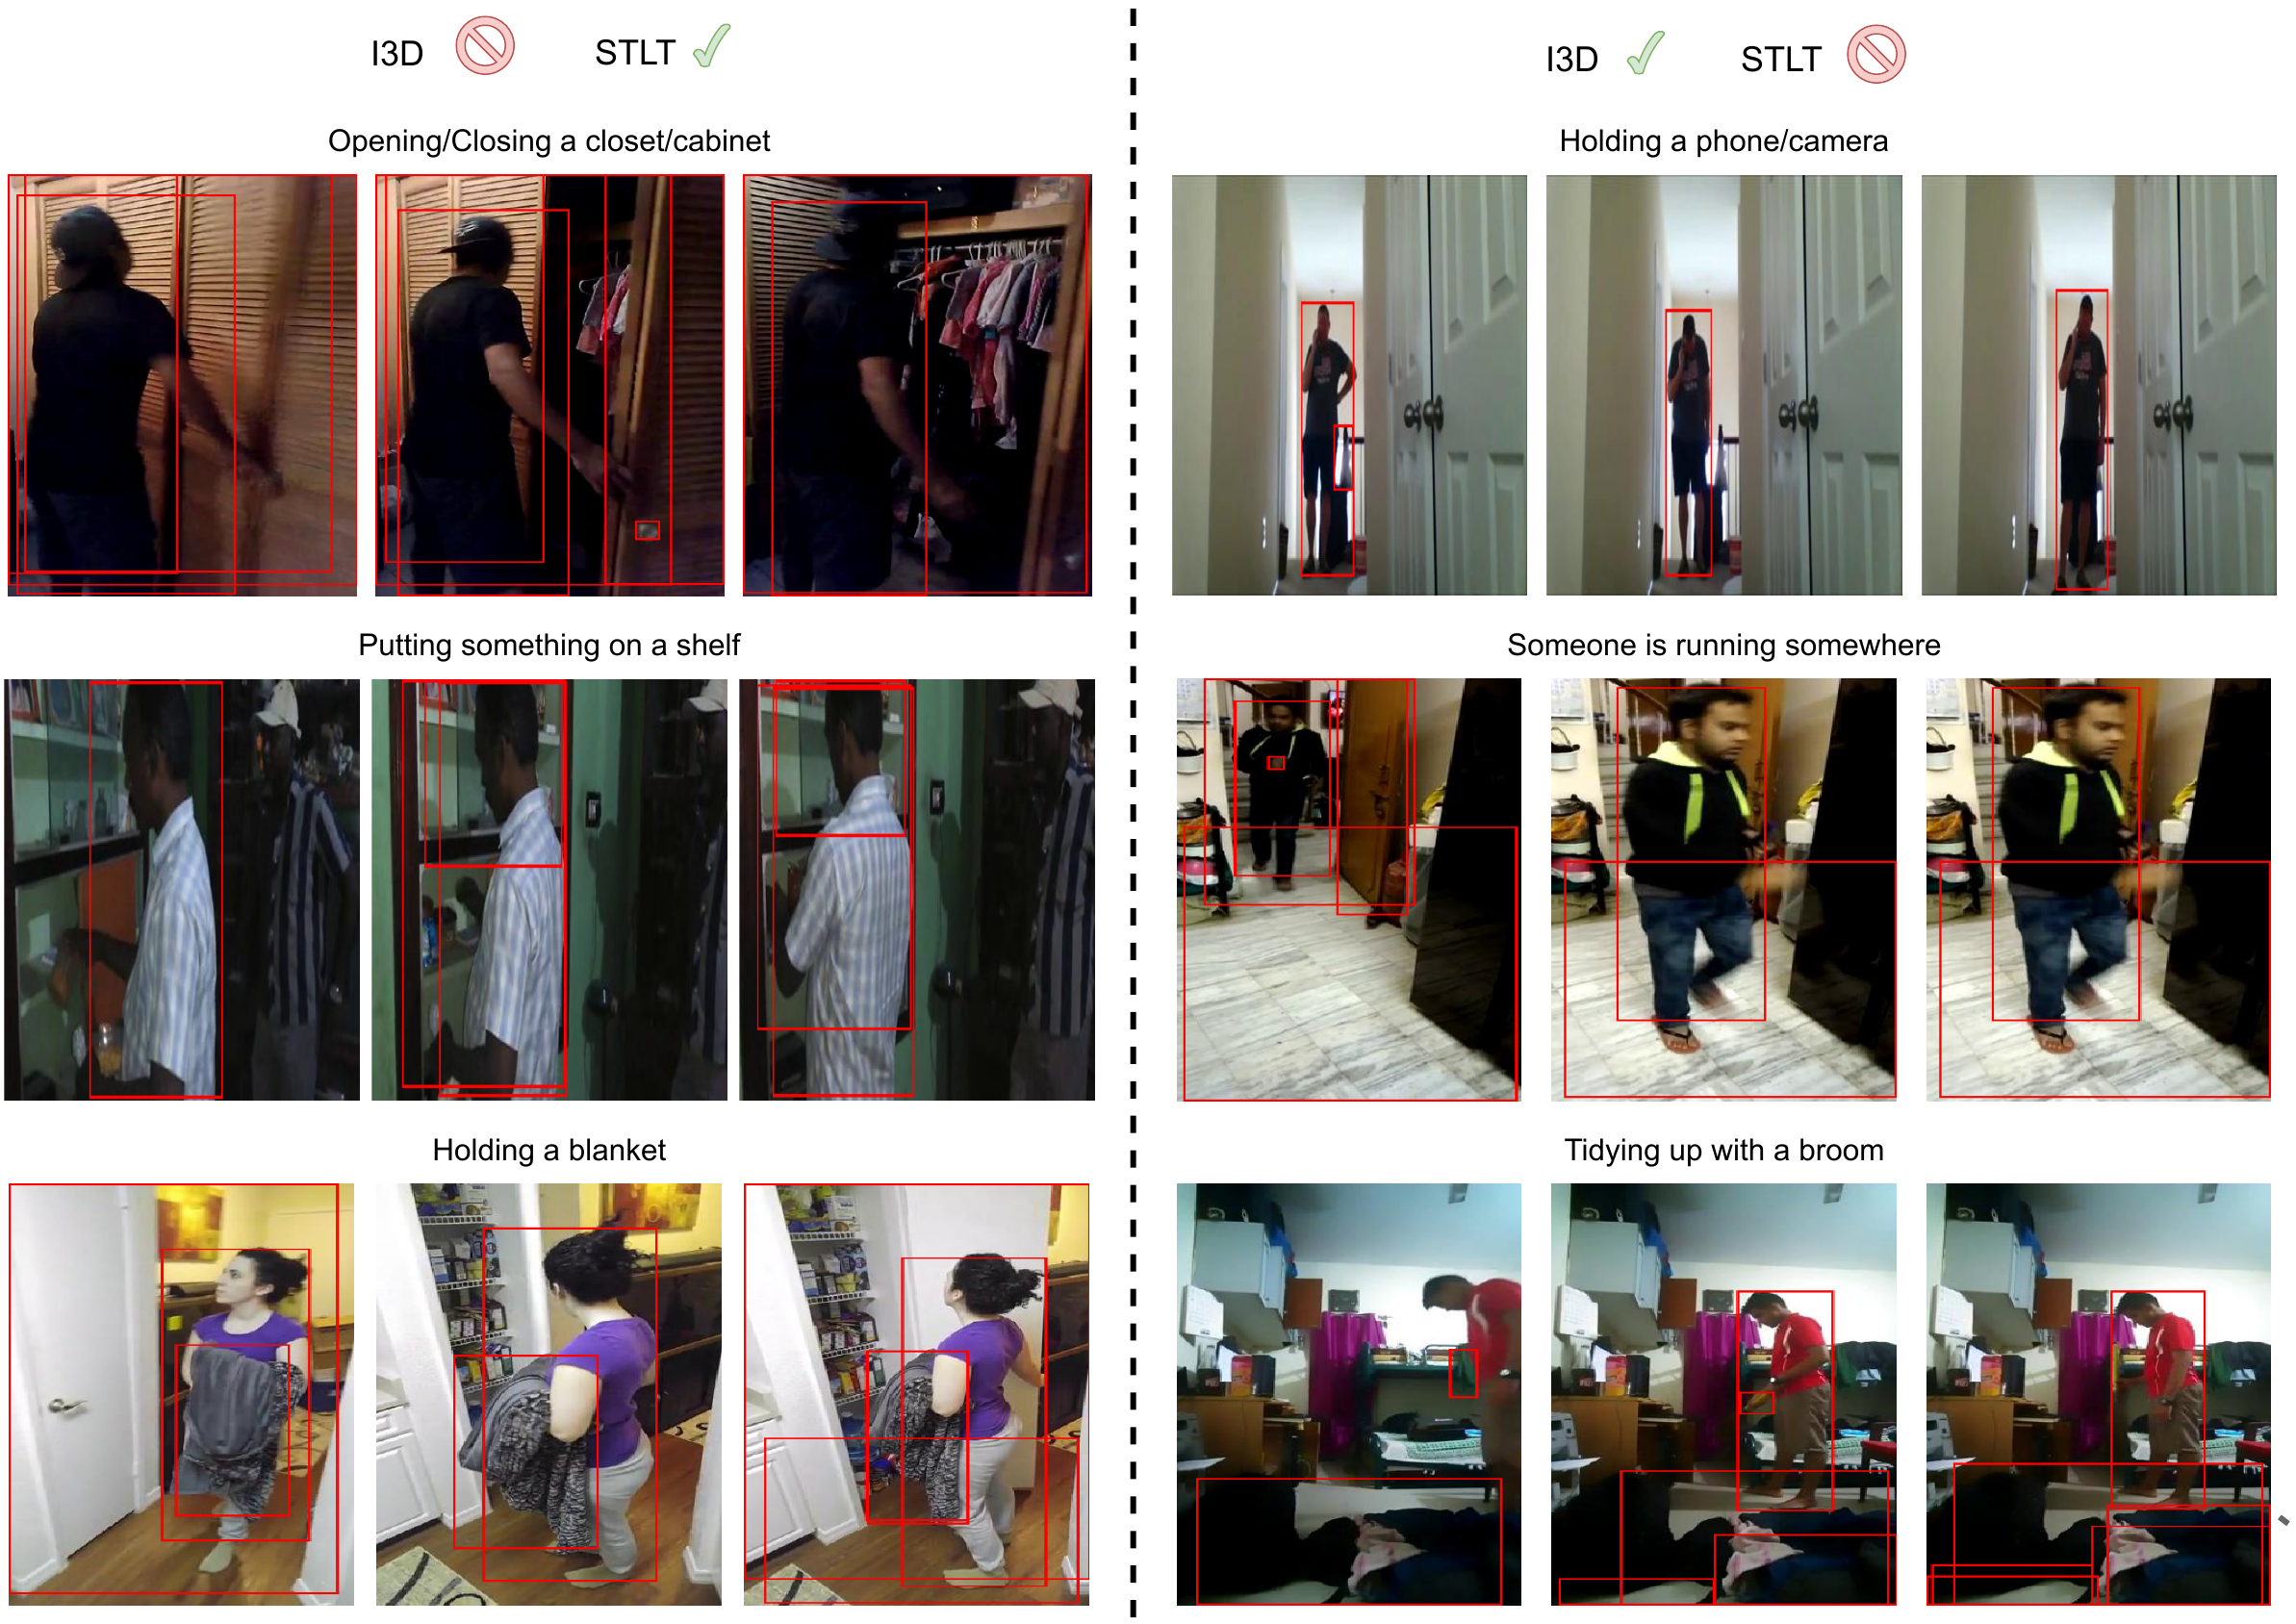}
\caption[Qualitative evaluation on the Action Genome.]{Qualitative evaluation on the Action Genome. \textbf{Left:} I3D mispredicts, STLT predicts correctly. \textbf{Right:} STLT mispredicts, I3D predicts correctly. Above each set of 3 video frames is the ground truth action class.}
\label{bmvc2021:appendix:fig:qualitative-actiongenome-appendix}
\end{figure*}

We provide an additional qualitative evaluation on the Something-Else compositional split. We follow the same setup as in Figure~\ref{bmvc2021:fig:qualitative}, where we are interested in visually inspecting three error types:
\begin{inparaenum}[(i)]
\item R3D predicts wrong, \blackgls{stlt} predicts correct action;
\item STLT predicts wrong, R3D predicts correct action;
\item STLT and R3D predict wrong, \blackgls{cacnf} predicts correct action.
\end{inparaenum}
We show the results in Figure~\ref{bmvc2021:appendix:fig:qualitative-smth-appendix}.\par
Lastly, we visually inspect how STLT copes with background clutter, and plot two error types:
\begin{inparaenum}[(i)]
\item I3D predicts the correct action with a probability less than 0.5, STLT predicts the correct action with a probability higher than 0.5;
\item STLT predicts the correct action with a probability less than 0.5, and I3D predicts the correct action with a probability higher than 0.5.
\end{inparaenum}
Note that in both scenarios, we show the frames where the action of interest occurred, i.e., the action for which there is a mismatch between the model's predictions. Note that there may be other actions occurring simultaneously, or in other parts of the video. The results are shown in Figure~\ref{bmvc2021:appendix:fig:qualitative-actiongenome-appendix}.
