# Supplementary material for: Bridging Modalities and Transferring Knowledge: Enhanced Multimodal Understanding and Recognition
Source: arXiv:2512.20501 source file (2025-12-23)
Supplement: Supplementary file 2 [file conll2020_appendix.tex]

\chapter{Appendix for Translating Medical Text into Locations in a 3D Human Atlas}\label{ch:conll2020-appendix}
The Supplementary material is organized as follows:

\begin{itemize}
    \item Details on the Human Atlas (\S\ref{conll2020:appendix:sec:human_atlas}).
    \item Details about the metrics we use to evaluate the human atlas grounding (\S\ref{conll2020:appendix:sec:metrics}).
    \item Implementation details (\S\ref{conll2020:appendix:sec:experimental-setup}).
    \item Ablation study on temperature terms and sampled voxel points (\S\ref{conll2020:appendix:sec:hyperparams}).
    %\item Quantifying the motivation: co-occurrences between functionally similar organs (\S\ref{conll2020:appendix:sec:coocurrences}).
\end{itemize}

\section{Human Atlas}\label{conll2020:appendix:sec:human_atlas}
There are multiple digital anatomical models available. The Virtual Population \cite{christ2009virtual, gosselin2014development} of the \textit{IT'IS Foundation}\footnote{\url{www.itis.swiss/}} contains anatomical models of 10 different persons obtained from MRI procedures. The \textbf{S}egmented \textbf{I}nner \textbf{O}rgans \textbf{(SIO)} from the \textit{Voxel-Man} project \cite{hohne2001realistic, pommert2001creating, schiemann1997segmentation} \footnote{\url{www.voxel-man.com/}} is based on the \textit{Visible Human Male} (U.S. National Library of Medicine \footnote{\url{www.nlm.nih.gov/research/visible/}}) and contains 202 labeled anatomical objects within the human torso. The model consists of 774 slices obtained by CT and MRI imaging, where each slice contains a cryosection image, a CT image, and a segmentation label image where the grayscale level corresponds to a segmentation label of the tissue (Figure~\ref{conll2020:appendix:fig:voxelman}).

\begin{figure}
\centering
\includegraphics[width=\textwidth,scale=0.5]{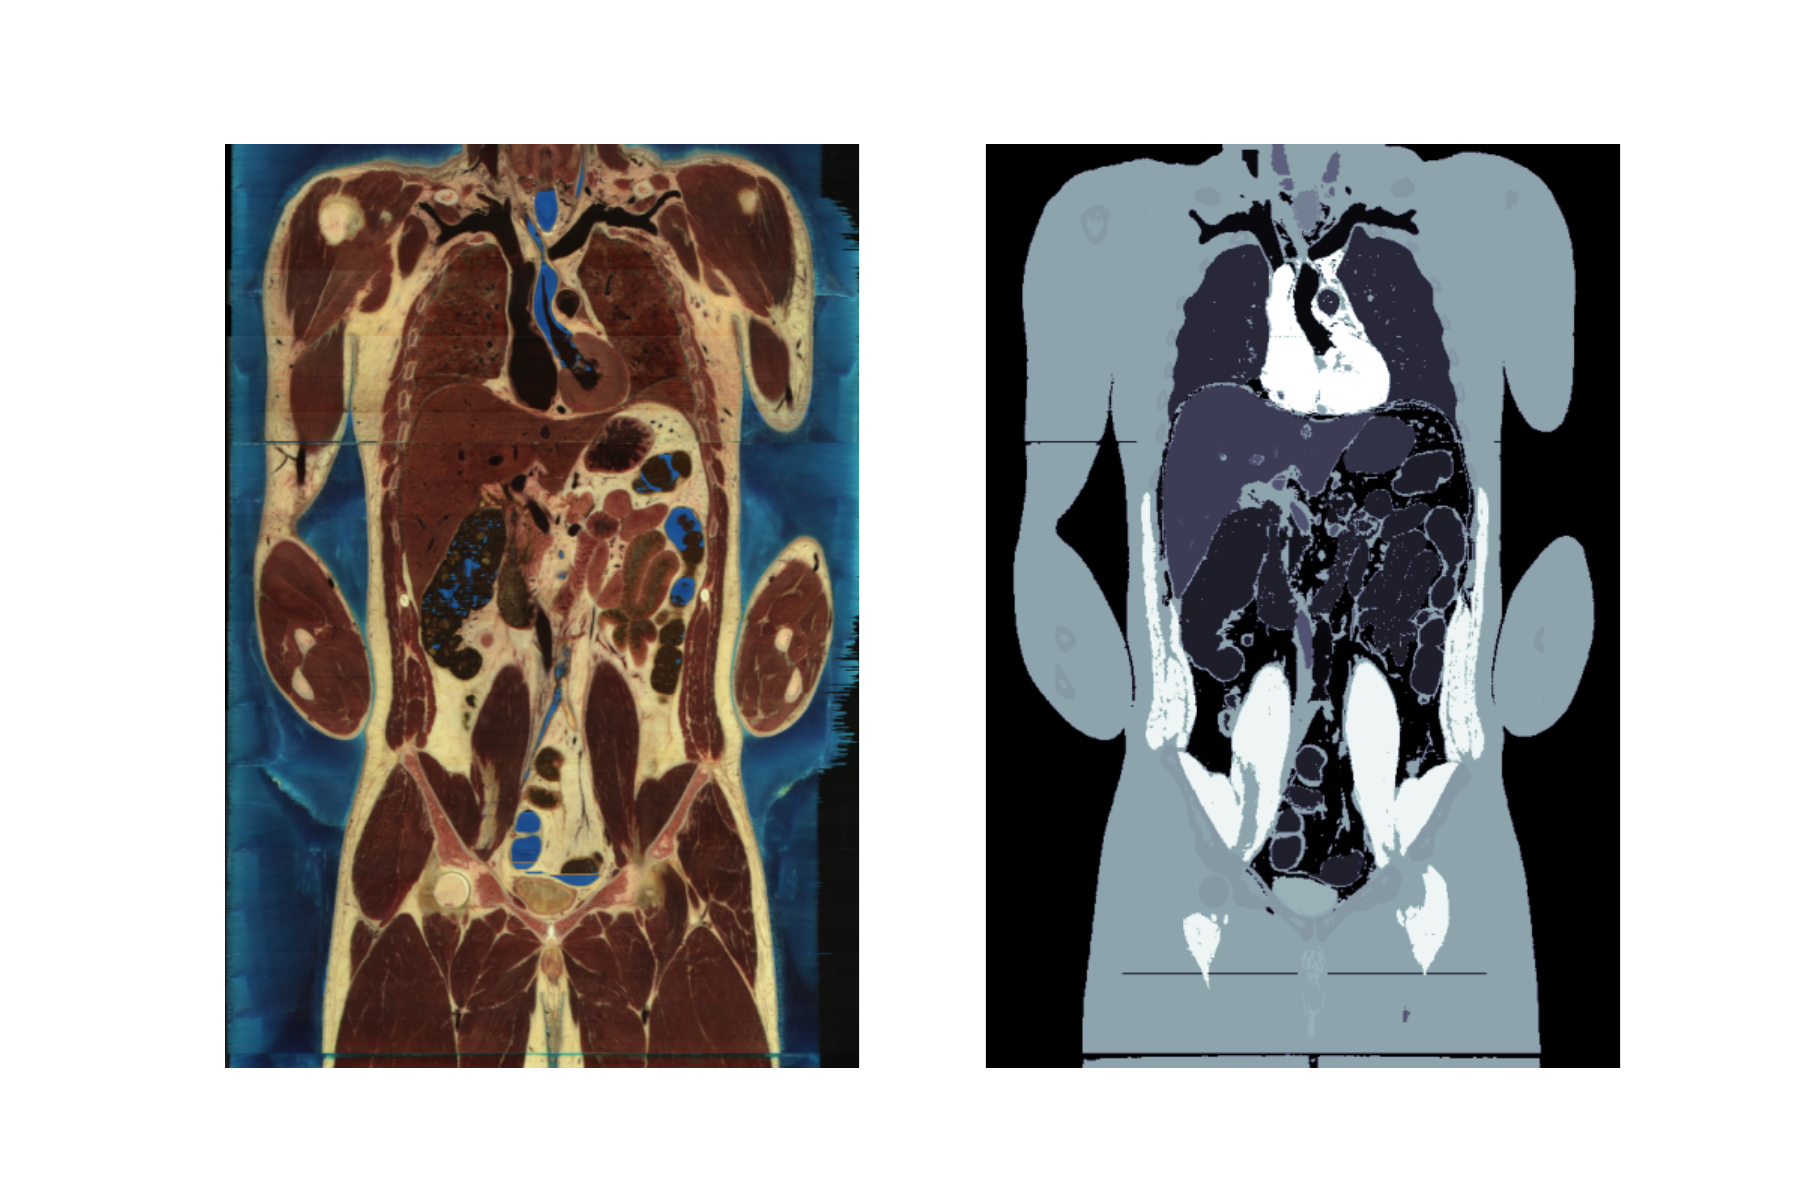}
\caption[Cross-sections of the RGB and grayscale volume representing segmentation labels.]{Cross-sections of the RGB (left) and grayscale volume (right) representing segmentation labels \cite{pommert2001creating}.}
\label{conll2020:appendix:fig:voxelman}
\end{figure}

The Segmented Inner Organs (SIO) contains a glossary of medical terms and their associated segmentation labels. A list of synonyms and closely related word forms for each glossary term were retrieved. The ScispaCy UmlsEntityLinker \cite{Neumann2019ScispaCyFA} was used for searching the UMLS Metathesaurus \textit{(The Unified Medical Language System)} \cite{bodenreider2004unified} for all word forms of the SIO glossary\footnote{ScispaCy version 0.2.3 and en\_core\_sci\_lg pipeline}. The parameters of the UmlsEntityLinker were kept at default values.

SIO includes 202 anatomical objects with their distinct segmentation labels. Tissues such as skin, gray matter, white matter, and unclassified tissues were removed from the set of labeled terms, as they denote general medical concepts not characterized by specific compact locations in the human body. The vertebrae, bones, and muscles of the locomotor system were discarded as well. The blood vessels, being small, elongated, and often not particular to any single region of the body, were also removed. Additionally, we remove the remaining small organs with fewer than 1000 associated voxels. The SIO includes the model of the human head as well, which we do not use. 

In the case of categories for bilateral organs located symmetrically on both the left and the right side of the body, which are seldom mentioned explicitly in the texts, only the atlas voxels pertaining to the left organ were kept for every bilateral pair. Atlas labels that appear infrequently in medical literature, but are functionally related to other, more frequently occurring organs, or are colloquially referred to under a single, umbrella term, were merged. The aforementioned steps reduced the list of distinct anatomical objects of interest to 27: ``ampulla'', ``bronchi'', ``caecum'', ``diaphragm'', ``gallbladder'', ``larynx'', ``liver'', ``myocardium'', ``pancreas'', ``pericardium'', ``prostate'', ``rectum'', ``seminal gland'', ``small intestine'', ``spleen'', ``testis'', ``thyroid gland'', ``urinary bladder'', ``stomach'', ``colon'', ``penis'', ``trachea'', ``ventricle'', ``atrium'', ``kidney'', ``lung'', ``duodenum''.

% \section{Dataset}\label{conll2020:appendix:sec:dataset}
% Focusing on the articles pertaining to the human anatomy, we remove the samples that contain any of the following MeSH terms: "Animals",  "Rats", "Mice",  "Rats, Sprague-Dawley", "Rats, Wistar", "Mice, Inbred C57BL", "Rats, Inbred Strains", "Disease Models, Animal", "Dogs", "Rabbits", "Swine", "Mice, Inbred BALB C", "Guinea Pigs", "Mice, Knockout", "Cattle", "Animals, Newborn", "Mice, Transgenic", "Chickens",  "Sheep", "Mice, Inbred Strains", "Rats, Inbred F344", which typically correspond to articles that describe clinical trials on animals. Subsequently, we discard the MeSH terms which are not a name or a synonym of an atlas organ.

\section{Metrics}\label{conll2020:appendix:sec:metrics}
For the IOR, the predicted 3D point lies inside the organ volume (\textit{hit}) when its coordinates, rounded to the nearest integer to represent voxel indices, are within the set of indices of voxels that make up the corresponding organ.  However, in the case of hollow organs, such as the intestines and the stomach, scoring a \textit{hit} would require predicting a point that lies exactly within a (usually very thin) organ wall, as the region of the organ's lumen is typically not included. Therefore, we use a more relaxed criterion, and record a \textit{hit} when the predicted 3D point is inside or sufficiently close to the organ volume, which we consider to be the case when its coordinates are less than 1cm away from the nearest voxel of the target organ. In cases of multiple target organs, we measure a \textit{hit} when the predicted coordinates lie within or sufficiently close to any one of the given organs.

When the projection is exactly inside the volume of the organ, the NVD is zero, and otherwise, it is measured as the distance to the surface of the nearest organ in the text. The NVD-O metric complements the NVD metric, such that it gives insight into how far off the prediction is when it misses the correct organ.

% \section{Qualitative Example of Ovaries}\label{conll2020:appendix:sec:qualitative}

% The Wikipedia paragraph describing the structure of the ovaries \footnote{\url{https://en.wikipedia.org/wiki/Ovary}}:
% \textit{"The ovaries are considered the female gonads. Each ovary is whitish in color and located alongside the lateral wall of the uterus in a region called the ovarian fossa. The ovarian fossa is the region that is bounded by the external iliac artery and in front of the ureter and the internal iliac artery. This area is about 4 cm x 3 cm x 2 cm in size. The ovaries are surrounded by a capsule, and have an outer cortex and an inner medulla. The capsule is of dense connective tissue and is known as the tunica albuginea. Usually, ovulation occurs in one of the two ovaries releasing an egg each menstrual cycle. The side of the ovary closest to the fallopian tube is connected to it by infundibulopelvic ligament, and the other side points downwards attached to the uterus via the ovarian ligament. Other structures and tissues of the ovaries include the hilum."}

% The first sentence - ``The ovaries are considered the female gonads", was removed, as it mentions the term \textit{gonads}, which is a strong clue for the model, as the male gonad (``testis''), was present in the atlas. 

\section{Implementation Details}\label{conll2020:appendix:sec:experimental-setup}
We use \textsc{Bert\textsubscript{Base}} \cite{devlin2018bert} as the backbone of the trained models. We use AdamW \cite{loshchilov2017decoupled} with a learning rate of $10^{-5}$ as per Devlin~\etal~\cite{devlin2018bert}, weight decay of $10^{-2}$ and clip the gradients when the global norm exceeds 2.0. We perform early stopping by saving the model with the best performance on the validation set. We only tune the hyperparameters related to the \blackgls{sod} loss function, and we keep everything else fixed as per the standard practice \cite{devlin2018bert}. Our implementation uses PyTorch \cite{paszke2019pytorch} and the HuggingFace Transformers library \cite{wolf2019transformers}.

\section{Ablation Study: Varying Temperatures and Sampled Voxels}\label{conll2020:appendix:sec:hyperparams}
Table \ref{conll2020:appendix:table:temperatures-100-points} and \ref{conll2020:appendix:table:temperatures-1000-points} showcase how varying the temperature terms $\gamma_p$ and $\gamma_o$ affect the results measured by \blackgls{ior}, \blackgls{nvd} and \blackgls{nvdo} on the full test set of medical articles. In particular, Table \ref{conll2020:appendix:table:temperatures-100-points} shows the results when the model is trained with 100 voxel points sampled for each organ during training, while table \ref{conll2020:appendix:table:temperatures-1000-points} shows the results when the model is trained by sampling 1000 voxel points during training.

\begin{table}[t]
\centering
\resizebox{0.8\textwidth}{!}{
\begin{tabular}{lccc} \toprule
{Method} & {IOR} & {NVD} & {NVD-O} \\ \midrule
$\gamma_p$ = 0.1, $\gamma_o$ = 0.1 & 89.2 $\pm$ 0.5 & 0.9 $\pm$ 0.1 & 2.8 $\pm$ 0.1 \\
$\gamma_p$ = 0.1, $\gamma_o$ = 0.5 & 88.8 $\pm$ 0.5 & \textbf{0.8 $\pm$ 0.1} & 2.7 $\pm$ 0.2 \\
$\gamma_p$ = 0.1, $\gamma_o$ = 1.0 & \textbf{89.4 $\pm$ 0.5} & \textbf{0.8 $\pm$ 0.1} & 2.5 $\pm$ 0.2 \\
$\gamma_p$ = 0.5, $\gamma_o$ = 0.1 & 82.5 $\pm$ 0.6 & 1.0 $\pm$ 0.1 & 2.3 $\pm$ 0.1 \\
$\gamma_p$ = 0.5, $\gamma_o$ = 0.5 & 86.7 $\pm$ 0.5 & 0.9 $\pm$ 0.1 & 2.1 $\pm$ 0.1 \\
$\gamma_p$ = 0.5, $\gamma_o$ = 1.0 & 85.0 $\pm$ 0.6 & 1.0 $\pm$ 0.1 & 2.3 $\pm$ 0.1 \\
$\gamma_p$ = 1.0, $\gamma_o$ = 0.1 & 83.6 $\pm$ 0.6 & 1.0 $\pm$ 0.1 & 2.4 $\pm$ 0.1 \\
$\gamma_p$ = 1.0, $\gamma_o$ = 0.5 & 82.2 $\pm$ 0.6 & 1.0 $\pm$ 0.1 & 2.3 $\pm$ 0.1 \\
$\gamma_p$ = 1.0, $\gamma_o$ = 1.0 & 82.2 $\pm$ 0.6 & 1.0 $\pm$ 0.1 & \textbf{1.9 $\pm$ 0.1} \\ \bottomrule
\end{tabular}
}
\caption[Experiments with 100 sampled voxels during training.]{Results on the full test set from models trained with varying inference while randomly sampling 100 voxels during training.}
\label{conll2020:appendix:table:temperatures-100-points}
\end{table}

\begin{table}[t]
\centering
\resizebox{0.8\textwidth}{!}{
\begin{tabular}{lccc} \toprule
{Method} & {IOR} & {NVD} & {NVD-O} \\ \midrule
$\gamma_p$ = 0.1, $\gamma_o$ = 0.1 & 89.1 $\pm$ 0.5 & 1.0 $\pm$ 0.1 & 3.6 $\pm$ 0.2 \\
$\gamma_p$ = 0.1, $\gamma_o$ = 0.5 & \textbf{89.3 $\pm$ 0.5} & \textbf{0.8 $\pm$ 0.1} & 2.5 $\pm$ 0.2 \\
$\gamma_p$ = 0.1, $\gamma_o$ = 1.0 & 89.2 $\pm$ 0.5 & \textbf{0.8 $\pm$ 0.1} & 2.4 $\pm$ 0.2 \\
$\gamma_p$ = 0.5, $\gamma_o$ = 0.1 & 84.0 $\pm$ 0.6 & 1.0 $\pm$ 0.1 & 2.6 $\pm$ 0.2 \\
$\gamma_p$ = 0.5, $\gamma_o$ = 0.5 & 86.8 $\pm$ 0.5 & 0.9 $\pm$ 0.1 & \textbf{2.0 $\pm$ 0.1} \\
$\gamma_p$ = 0.5, $\gamma_o$ = 1.0 & 84.0 $\pm$ 0.6 & 0.9 $\pm$ 0.1 & \textbf{2.0 $\pm$ 0.1} \\
$\gamma_p$ = 1.0, $\gamma_o$ = 0.1 & 84.2 $\pm$ 0.6 & 1.1 $\pm$ 0.1 & 2.8 $\pm$ 0.2 \\
$\gamma_p$ = 1.0, $\gamma_o$ = 0.5 & 81.4 $\pm$ 0.6 & 1.0 $\pm$ 0.1 & 2.1 $\pm$ 0.1 \\
$\gamma_p$ = 1.0, $\gamma_o$ = 1.0 & 83.1 $\pm$ 0.6 & 1.0 $\pm$ 0.1 & 2.1 $\pm$ 0.1 \\ \bottomrule
\end{tabular}
}
\caption[Experiments with 1000 sampled voxels during training.]{Results on the full test set from models trained with varying inference while randomly sampling 1000 voxels during training.}
\label{conll2020:appendix:table:temperatures-1000-points}
\end{table}
