# Supplementary material for: Bridging Modalities and Transferring Knowledge: Enhanced Multimodal Understanding and Recognition
Source: arXiv:2512.20501 source file (2025-12-23)
Supplement: Supplementary file 3 [file emnlp2020_appendix.tex]

\chapter{Appendix for Translating Text-Based Spatial Relations to 2D Spatial Arrangements}\label{ch:emnlp2020-appendix}
The Supplementary material is organized as follows:

\begin{itemize}
    \item Details on the Recurrent Neural Network baselines (\S\ref{emnlp2020:appendix:sec:rnn_baseline}).
    \item Details on the data augmentation (\S\ref{emnlp2020:appendix:sec:augmentation}).
    \item Implementation details (\S\ref{emnlp2020:appendix:sec:experimental-setup}).
    \item Additional qualitative evaluation (\S\ref{emnlp2020:appendix:sec:qualitative}).
\end{itemize}

\section{Recurrent Neural Network Baselines}\label{emnlp2020:appendix:sec:rnn_baseline}
The recurrent neural network baselines consist of two bidirectional GRU recurrent neural networks \cite{cho2014learning}, each with a hidden size of 256, where one is used for obtaining contextual embeddings of the text and the other for the clip-arts. Prior to the RNN, the clip-arts are ordered according to the HO, and an embedding of size 256 is obtained for every clip-art and word in the sentences. In both models, an attention module attends on every sentence word with respect to every clip-art in a sequential manner when generating the spatial arrangements of that clip-art. The Attention + Rnn baseline, uses an extra GRU recurrent neural network for propagating contextual information of the generated spatial arrangements. The hidden size of the attention module is kept the same as in the \blackgls{gru} recurrent neural network (256 dimensional). Both models are trained for 300 epochs with a fixed learning rate of $2e-5$, while the model with the best performance on the validation set is used for inference on the test set. There are no other forms of regularization. As in \blackgls{sr-bert}, we implement two variants of the Attention and Attention+Rnn models, namely a continuous and a discrete version.

\section{Data Augmentation}\label{emnlp2020:appendix:sec:augmentation}
Due to the limited size of the dataset, we employ several data augmentation strategies to artificially increase the quantity of data, while preserving the meaning of each abstract scene. Furthermore, we want to impose greater importance on the relative positioning of the elements and obtain a model that is invariant on whether the scenes are mirrored across the y-axis and invariant on the order of the sentences from the scene descriptions.
% To this end, the data augmentations we use are:

\begin{itemize}
    \item Note that in the Abstract Scenes dataset, each scene is paired with a set of $\sim6$ sentences, where each sentence is entirely self-contained (e.g., ``The cat is on the bench''). For that reason, we conclude that the order of the sentences does not affect the semantic meaning of the scenes, and randomly shuffle the sentences before providing them as input to the models.
    \item For each scene in the dataset, the mirrored scene across the $y$ axis is also valid. Therefore, we randomly mirror each scene with 50\% probability by inverting the $x$ coordinates and the orientation of the clip-arts.
    % - $\left| width - x \right|$, and reverting the orientation - $\left| 1 - o \right|$ of each object.
    \item With 50\% probability we move all elements in the scene up, down, left, or right, by a random number of quantization intervals, with 25\% probability for each movement. The number of quantization intervals is sampled uniformly from $[0, w]$ for $x$ and $[0, h]$ for $y$, where $w$ and $h$ are the scene width and height respectively.
\end{itemize}

\section{Implementation Details}\label{emnlp2020:appendix:sec:experimental-setup}
The backbone of all our models is a pre-trained \textsc{Bert\textsubscript{Base}} variant from Devlin~\etal~\cite{devlin2018bert}.
% , pre-trained on the BooksCorpus \cite{zhu2015aligning} and English Wikipedia.
We train all \blackgls{sr-bert} models using \blackgls{mpm} as a training objective for 300 epochs, while we train the clip-arts predictor model for 50 epochs. We use the AdamW \cite{kingma2014adam} optimizer with a learning rate of $2e-5$ for training the \textsc{SR-Bert} models and the clip-art predictor models.
% since it sped up convergence significantly.
For all \textsc{SR-Bert} models, we empirically set the scaling factor $\lambda$ to $\frac{1}{3}$ to obtain the average of the three spatial embeddings. Apart from applying early stopping, i.e., saving the model with the best performance on the validation set, we do not tune our hyperparameters.
% Since we use a fixed quantization interval ($\text{bin\_size}=20$), $w=25$ is equal to 25, and $h=20$, on a scene size of $500 \times 400$.
We use a separate decoding strategy during model selection on the validation set, so that we can make an unbiased estimate about the performance of the decoding strategies (\S\ref{emnlp2020:sec:decoding-strategies}). Namely, when performing inference on the validation set, we generate the spatial arrangement of each scene element by conditioning it on the ground truth spatial positions of all other scene elements in addition to the sentences. The deep learning library of choice is PyTorch \cite{paszke2019pytorch} alongside the HuggingFace Transformers package \cite{wolf2019transformers}.

\section{Additional Qualitative Evaluation}\label{emnlp2020:appendix:sec:qualitative}
We select 10 random samples from the test and generate the spatial arrangements given the language using our two best models: discrete with HC decoding and continuous with HO decoding. We report the results in Figure~\ref{emnlp2020:appendix:fig:appendix_generated}.

\section{Additional Information About the User Study}
We conducted the user study on Amazon Mechanical Turk where for each assignment (generated scene) 3 distinct participants are voting for the spatial correctness of the sentences. One such assignment can be seen in Figure~\ref{emnlp2020:appendix:fig:userstudy-turk}. We collect the results from the user study such that in case a sentence has been selected as \textit{True} by at least two participants, we deem that sentence as \textit{True} for the scene, and \textit{False} otherwise. Then, for each scene, we measure the average number of accepted spatial arrangements as the fraction of accepted sentences for that scene. Finally, we obtain the macro-average over the whole subset of scenes.

\begin{figure}[t]
\centering
\includegraphics[width=1.0\columnwidth]{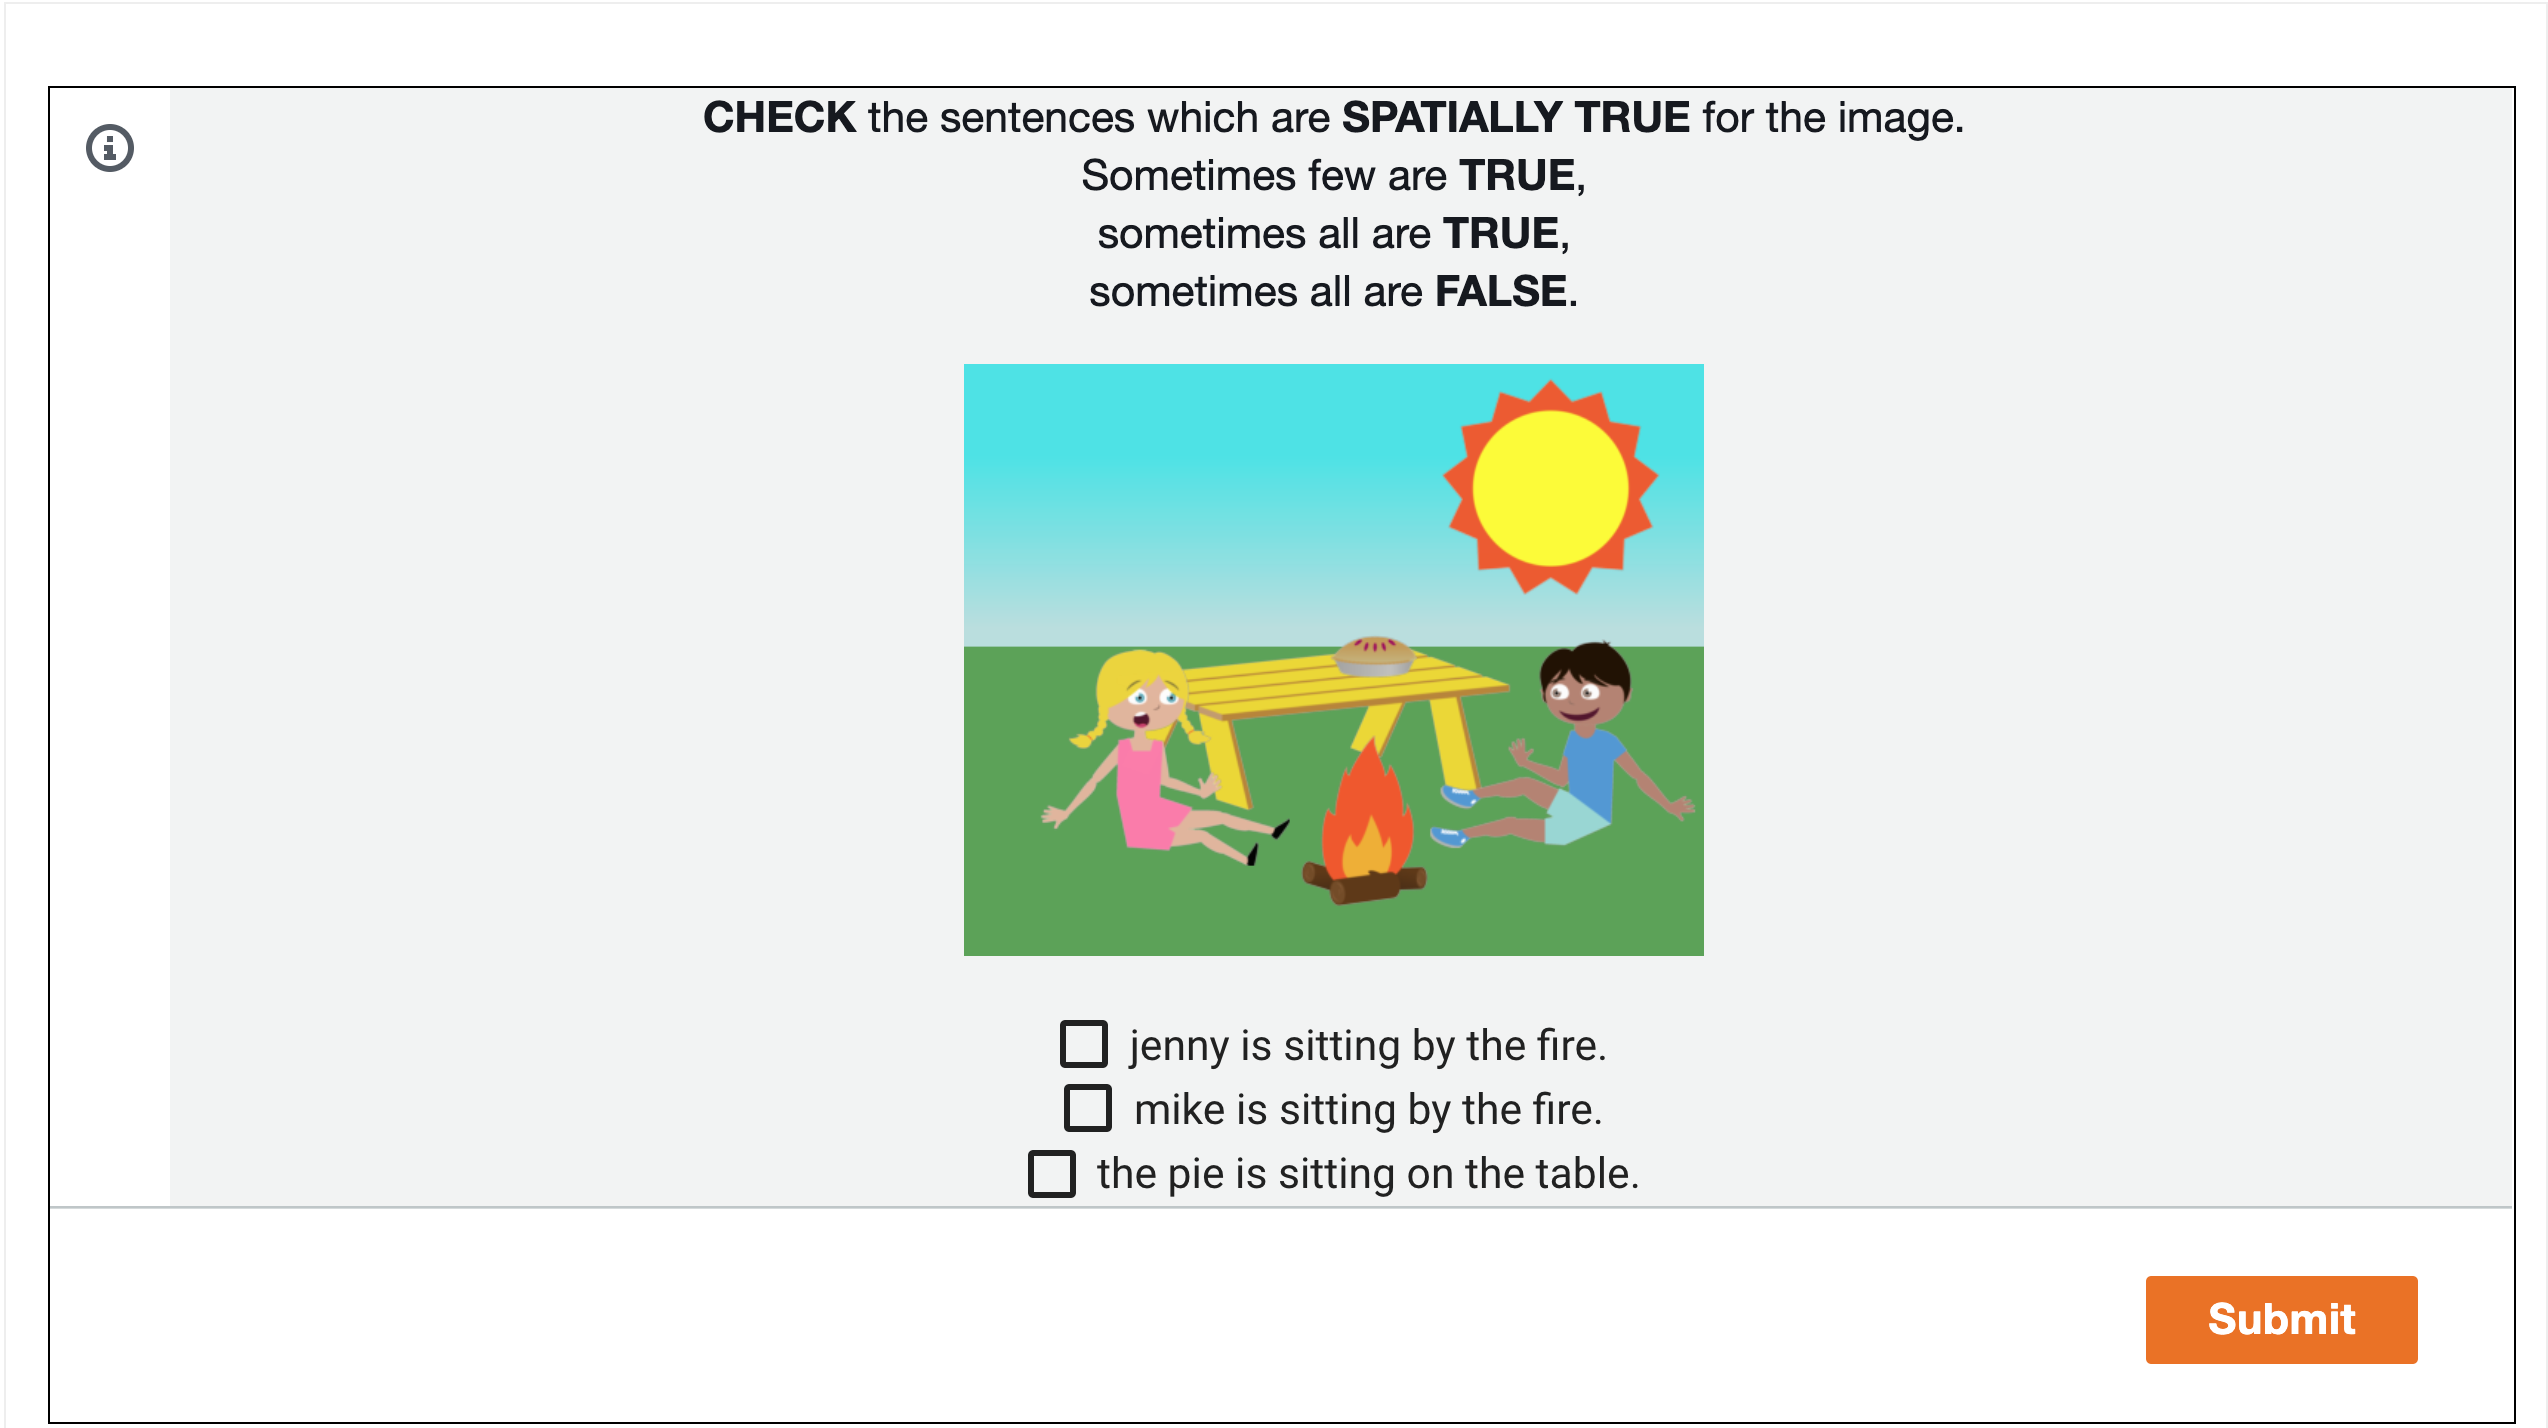}
\caption{Sample task of the user study on Amazon Mechanical Turk.}
\label{emnlp2020:appendix:fig:userstudy-turk}
\end{figure}

\begin{figure}[t]
\centering
\includegraphics[width=2.0\textwidth,height=1.0\textheight,keepaspectratio]{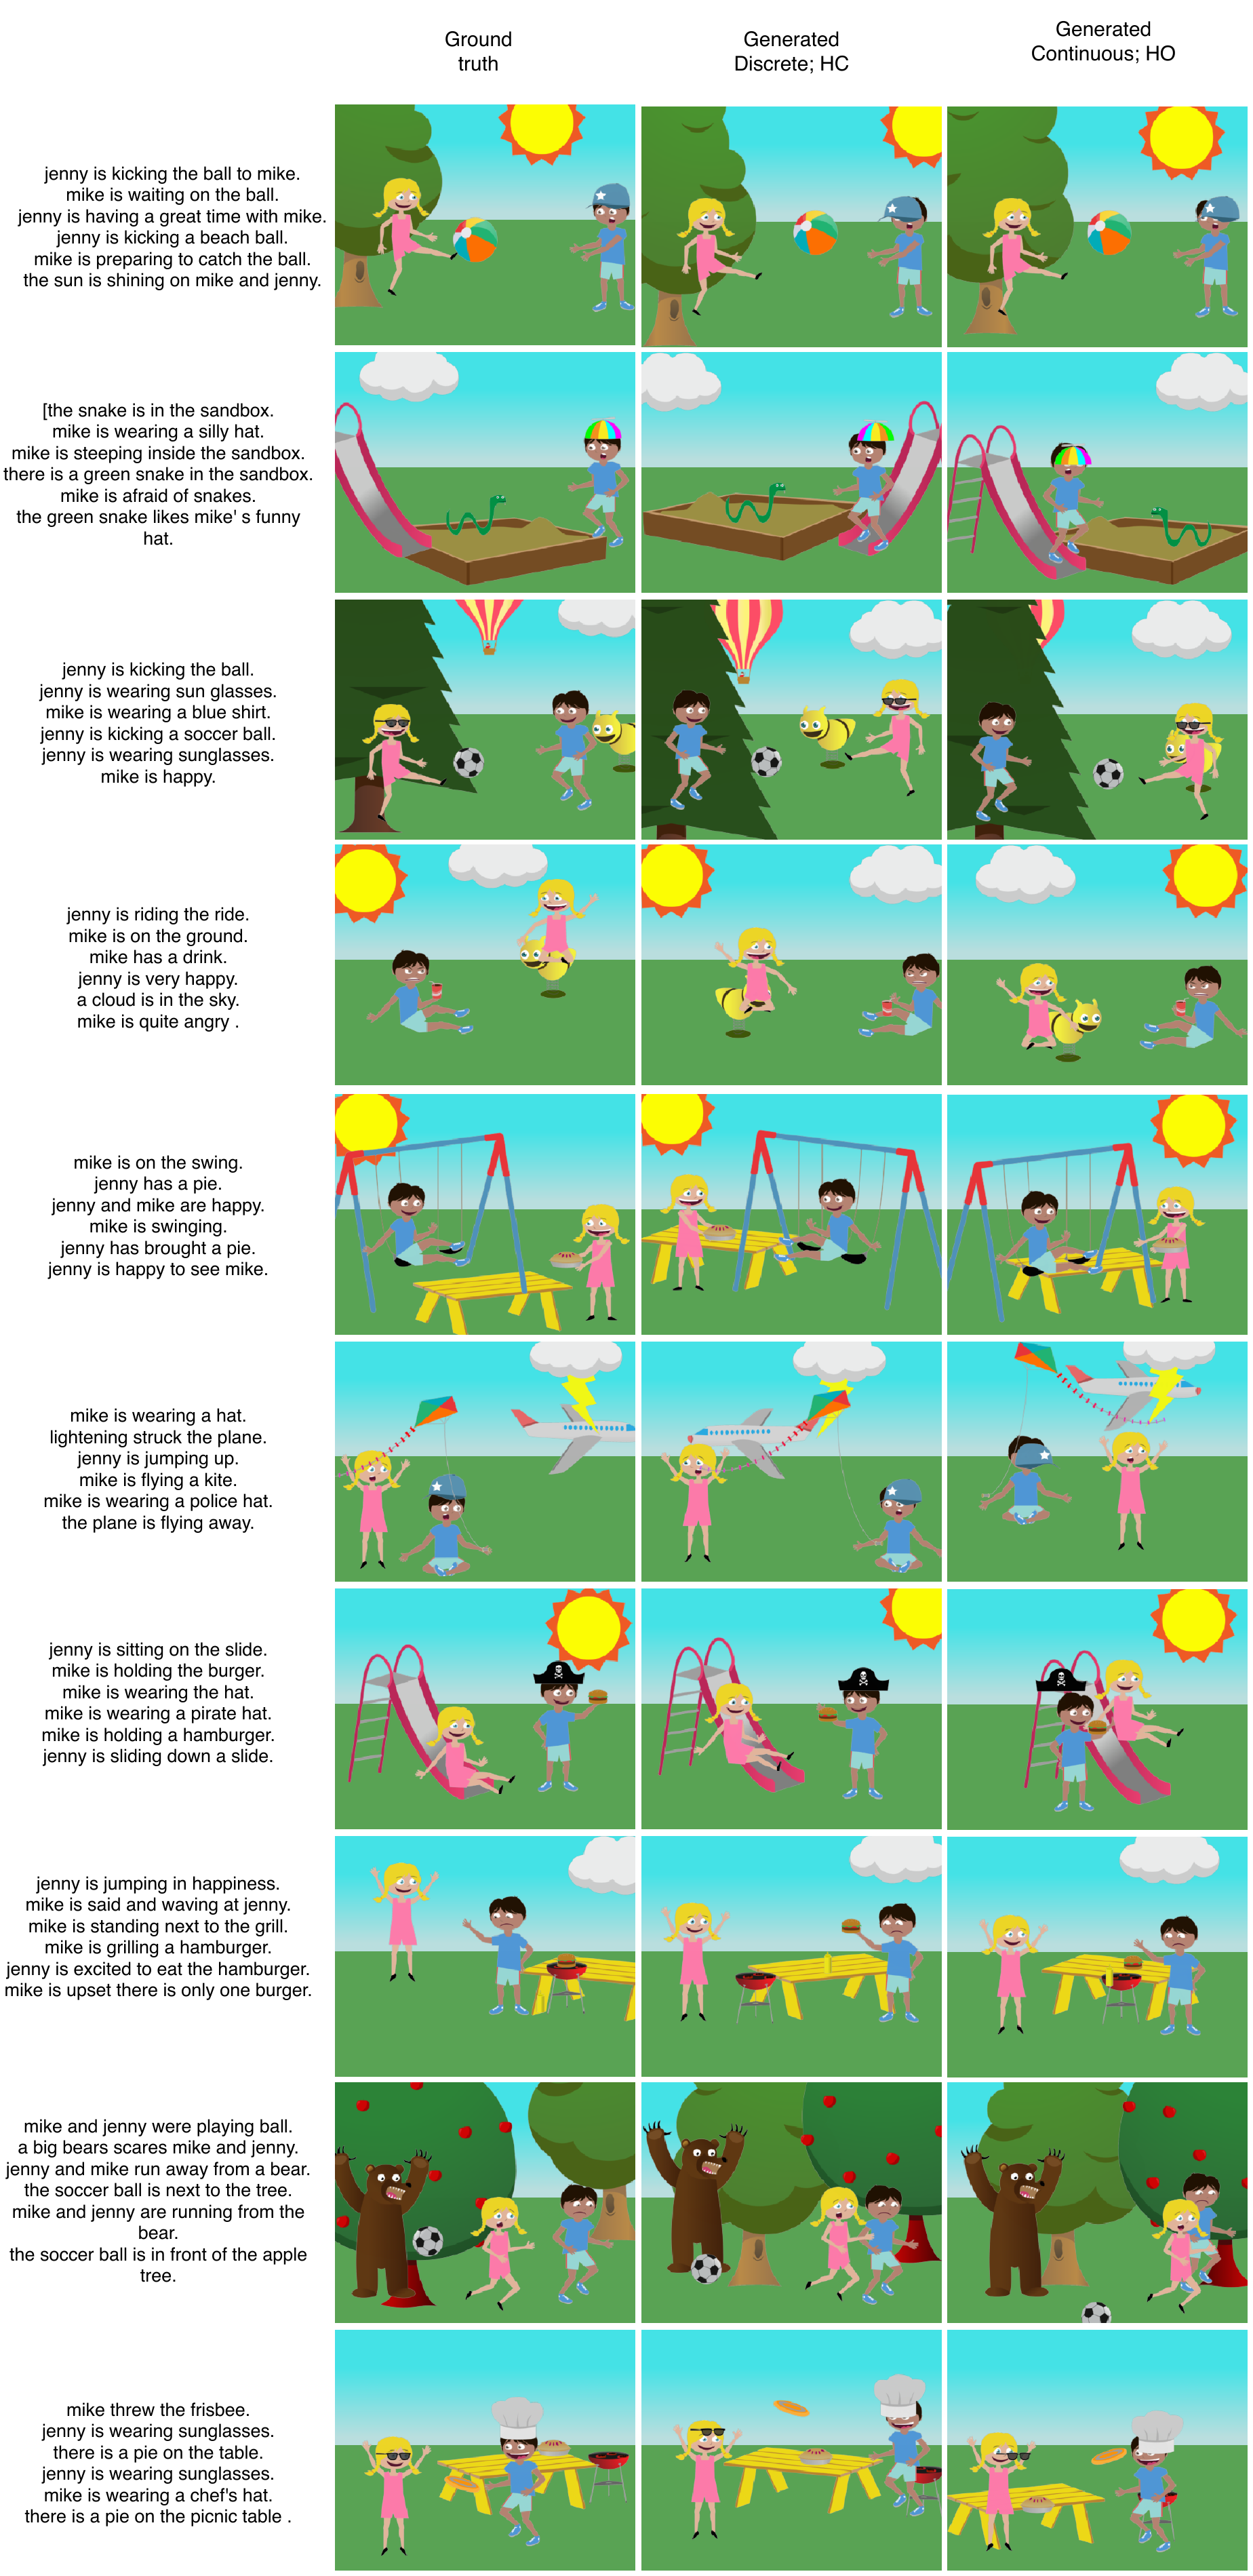}
\caption{Generated spatial arrangements conditioned on language on 10 random samples from the test set.} 
\label{emnlp2020:appendix:fig:appendix_generated}
\end{figure}

\cleardoublepage
