# Supplementary material for: Bridging Modalities and Transferring Knowledge: Enhanced Multimodal Understanding and Recognition
Source: arXiv:2512.20501 source file (2025-12-23)
Supplement: Supplementary file 4 [file emnlp2023_appendix.tex]

\chapter{Appendix for Translating Structured Text to Canonical Facts in Large-Scale Knowledge Graphs}
The Supplementary material is organized as follows:

\begin{itemize}
    \item Details on the Out-of-Knowledge Graph detection task (\S\ref{emnlp2023:appendix:out-of-kg}).
     \item Details on the Out-of-Knowledge Graph detection models (\S\ref{emnlp2023:appendix:out-of-kg-models}).
     \item Discussion on the data quality of \textbf{\blackgls{falb}} (\S\ref{emnlp2023:appendix:data-quality}).
     \item Implementation details (\S\ref{emnlp2023:appendix:experimental-setup}).
\end{itemize}

\section{Details on the Out-of-Knowledge Graph Detection Task}\label{emnlp2023:appendix:out-of-kg}
In \S\ref{emnlp2023:sec:out-of-kg-detection} we evaluate the ability of the models to detect whether an OIE slot (surface-form entity, or surface-form relation) is present in the Knowledge Graph. Intuitively, this task is more difficult than the OIE linking task, as the models need to generalize beyond the training data distribution to perform well on this task. Namely, when linking OIEs to a KG, all prior work \cite{zhang2019openki,jiang2021cori,wood2021integrating} makes the conjecture that the testing data (in the open world) is independent and identically distributed (i.i.d.) w.r.t.~the training data, which is an invalid assumption in certain scenarios. Notably, the Out-of-KG OIEs lie outside of the training data distribution. Therefore, a model that performs well on the OIE linking task does not warrant high performance on the Out-of-KG detection task. We observed that this is the case (i.e., a model performs well on the linking task, but performs poorly on the Out-of-KG task) when detecting out-of-KG relations.

Therefore, to ensure that the Out-of-KG data is indeed out-of-distribution (as it would be the case in practice), we impose the following constraints: (i) We select OIE-to-KG pairs from SynthIE, while the ``backbone'' model we build on top of is trained on REBEL; (ii) All entities and predicates---which are part of the KG facts from the testing data---are not in the KG at the time of training the \preranker.

To perform the evaluation, for each OIE slot we either leave its corresponding KG entry outside of the KG, and score a hit if the models predict a \textit{negative score} for that slot; or, we perform imputation of the Out-of-KG entries (thus, they are now part of the KG), and score a hit if the models predict a \textit{positive score} for that slot. Finally, we report the average accuracy over the two scenarios for each OIE slot. Note that, in this case, both micro- and macro-average yield the same number, because we have the same number of samples for each scenario.

\section{Out-of-Knowledge Graph Detection Models}\label{emnlp2023:appendix:out-of-kg-models}
All models that we use for the Out-of-KG detection task in \S\ref{emnlp2023:sec:out-of-kg-detection} are built on top of a \preranker, which is trained on REBEL. For all models, to obtain an out-of-KG indicator---True (1), or False (0)---we threshold the output of the models. For each model, we determine the optimal threshold (the confidence, or the entropy) on a hold-out validation dataset which we build on top of REBEL.

\paragraph{\textsc{Confidence@1-based heuristic:}} We obtain the KG links for each of the OIE slots using the \preranker. The linking is characterized by the cosine similarity between the embeddings of each OIE slot and the KG entries. We then compute the softmax of the top-5 highest cosine similarities, and finally threshold the confidence@1 to obtain a prediction; such that a confidence $< T_c$ indicates an out-of-KG instance, and a confidence $> T_c$ indicates an instance inside the KG, where $T_c$ is the confidence threshold. We use $T_c = [0.235; 0.260; 0.235]$ for detecting out-of-KG subjects, relations, and objects respectively.
\paragraph{\textsc{Entropy-based heuristic:}} Similar to the confidence@1-based method, we obtain the cosine similarities with the \preranker. However, instead of using the top-1 probability, we obtain the entropy of the top-5 predictions. We finally threshold the entropy to obtain a prediction, such that an entropy $> T_e$ indicates an out-of-KG instance, and an entropy $< T_e$ indicates an instance inside the KG, where $T_e$ is the entropy threshold. We use $T_e = [1.60; 1.58; 1.60]$ for detecting out-of-KG subjects, relations and objects respectively.
\paragraph{\textsc{Query-Key-Value Cross-Attention:}} Using the \preranker embeddings, we train a lightweight query-key-value cross-attention module on top with weights that are initialized with the identity matrix---at the start of training the \preranker embeddings are used as is. Given a query OIE slot embedding, the model attends over the KG entry embeddings representing the keys and values, and outputs a sigmoid normalized score (i.e., a probability) indicating the presence confidence of the OIE slot in the KG. During training, to obtain in-batch negatives, for each OIE slot we drop the KG entry counterpart with 50\% probability. We obtain additional negatives by sampling KG entries from the whole KG, which do not match any of the OIE slots in the batch. We train the model using the binary cross-entropy loss, such that, if the corresponding KG entry for an OIE slot is in the sampled KG subset, the model predicts a positive score averaged over the KG graph subset, and negative otherwise. We use a uniform threshold of $T_a = 0.3$ for all three slots.

\section{Data Quality}\label{emnlp2023:appendix:data-quality}
To assess FaLB's data quality, we performed a manual human evaluation. In particular, we did the following steps: 
\begin{enumerate}
    \item We randomly selected 100 data points, where each data point contained information about the provenance sentence, a KG fact that is contained in the sentence, and a corresponding OIE surface fact that was extracted from the sentence.
    \item Two expert annotators annotated each data point independently of whether the KG fact matches the OIE extraction semantically.
    \item We considered a data point as \emph{``correct''} only if the two annotators agreed that the KG fact semantically matches the information in the OIE triplet.
    \item We computed accuracy, inter-annotator agreement, and Kohen's kappa score. 
\end{enumerate}

We found that 97\% of the data points are considered \emph{``correct''} by both annotators. We also observed that the inter-annotator agreement was high: the annotators agreed in 99\% of the cases, with a high Kohen's kappa score \cite{mchugh2012interrater} of 0.80.
% Please refer to the supplementary material for the subset of samples that were provided to the expert annotators.

\section{Implementation details}\label{emnlp2023:appendix:experimental-setup}
We train all models for 10 epochs using AdamW with a learning rate of 5e-5 and weight decay of 1e-3. We use a RoBERTa \cite{liu2019roberta} model, distilled following the procedure of Sahn~\etal~\cite{sanh2019distilbert}. The model consists of 6 layers, a hidden size of 768, and has 12 self-attention heads. To reduce the computational complexity and memory demands, we further linearly project the embeddings obtained from the RoBERTa model to a 200-dimensional latent space. When training the \preranker models, we initialize the temperature $\tau$ to 0.07 as per Radford~\etal~\cite{radford2021learning}. We train \preranker models with negatives that are sampled from the whole KG, where we sample 128 negative KG entities and 64 negative KG predicates. When training the \reranker, we sample negatives such that we corrupt the slots of the KG fact by replacing them with incorrect ones. Instead of choosing the negatives at random, for each KG entry, we find its top 10 most similar KG entries, and sample negatives from this subset. This ensures that the \reranker model learns how to refine the predictions of the \preranker model. We implement everything using PyTorch \cite{paszke2017automatic}, while we use HuggingFace transformers \cite{wolf2019huggingface} for the RoBERTa implementation. Lastly, we use Faiss \cite{johnson2019billion} to enable fast linking to Knowledge Graphs.
