# Supplementary material for: Bridging Modalities and Transferring Knowledge: Enhanced Multimodal Understanding and Recognition
Source: arXiv:2512.20501 source file (2025-12-23)
Supplement: Supplementary file 5 [file iccv2023_appendix.tex]

\chapter{Appendix for Multimodal Knowledge Transference for Improving Egocentric Action Recognition}
The Supplementary material is organized as follows:

\begin{itemize}
    % \item Extended discussion and details regarding the datasets we use (\S\ref{iccv2023:appendix:datasets}).
    \item Additional details about each of the modalities and the modality-specific models we use (\S\ref{iccv2023:appendix:modalities}).
    % \item An ablation study, alike the one in Table~\ref{iccv2023:appendix:table_supp:ablation-weighting}, conducted on the Something-Something and Something-Else datasets (\S\ref{iccv2023:appendix:weighting}).
    \item Other approaches that perform multimodal transference for video action recognition (\S\ref{iccv2023:appendix:omnivore}).
    \item Implementation details (\S\ref{iccv2023:appendix:experimental-setup}).
    % \item Analysis of the performance of our approach on seen and unseen environments (\S\ref{iccv2023:appendix:epic_seen_unseen}).
    % \item Extended per-class performance breakdown for Epic-Kitchens and Something-Something (\S\ref{iccv2023:appendix:performance_breakdown}).
    % \item Learning curves on the Epic-Kitchens and Something-Something datasets (\S\ref{iccv2023:appendix:learning_curves}).
    % \item Additional qualitative examples on the Epic-Kitchens and the Something-Something datasets (\S\ref{iccv2023:appendix:qualitative_examples}).
\end{itemize}

\section{Data Modalities \& Models}\label{iccv2023:appendix:modalities}

\subsection{RGB frames}
To encode the RGB frames we follow the standard setting of Liu~\etal~\cite{liu2021swin} for all datasets -- Epic-Kitchens (including the Unseen split), Something-Something (including the Something-Else compositional generalization split). Unless stated otherwise, we use the \blackgls{swin_t} \cite{liu2021swin} model to process the RGB frames. During training, we resize the image such that the shorter dimension (typically the height) is set to a value randomly chosen from the interval $[224, 320]$, and subsequently select a random $224 \times 224$ crop. Additionally, we adopt random horizontal flips with probability $50$\% (only for Epic-Kitchens), and color jittering. During inference, we resize the image such that the shorter dimension (typically the height) is set to $224$, and then select a $224 \times 224$ central crop for each frame.

In the case of the 3D-Resnet \cite{kataoka2020would} models, where we focus on testing our approach on computationally cheaper and faster architectures and settings, we keep the same train and inference setup, with the exception of the final crop size which we reduce to $112$, as per Kataoka~\etal~\cite{kataoka2020would}.

\subsection{Optical Flow (OF)}
We process the optical flow frames in the same fashion as the RGB frames and use the same vision backbone (Swin-T) for both Epic-Kitchens (including the Unseen split) and Something-Something (including the Something-Else compositional generalization split). We use the two components of the velocity as the first two channels of the input. To maintain the same architecture, we append an additional channel where we set each pixel intensity to 0.0, effectively expanding the number of input channels to 3. We use the same data augmentations as with the RGB model, with the exception of color jitter. %We always use the Swin-T model as the backbone of our optical flow model.

\subsection{Audio (A)}
On Epic-Kitchens, we first convert the $24000$Hz stereo audio to $16000$Hz monoaural audio. We compute the mel-spectrograms of audio segments using 1024 FFT bins and 128 mel filter banks. We use the Hann window with a length of 160, with an 80 sample overlap between successive windows. We square the magnitude after computing the FFT, and thus obtain the signal power at each frequency bin for each time step. For the audio segments of $1.116$ with the sampling frequency of $16000$, we thus obtain spectrograms with $128$ frequency bins and $224$ timesteps.

During training, as data augmentation, we perform random time and frequency masking of the spectrograms, as per the work of Park~\etal~cite{park2019specaugment}. In time masking, with a probability of $50$\%, we randomly chose the number of masked time-steps $T_n$ from the range $[ 0, 80 ]$, and the starting time-step from the range $[ 0, 224 - T_n )$, such that, for all the frequency bins, the range of time-steps $[ T_s, T_s + T_n )$ is masked by setting the power value in the spectrogram to 0. In frequency masking, with a probability of $50$\%, we randomly chose the number of masked frequency bins $F_n$ from the range $[0, 80]$, and the starting frequency bin $F_s$ from the range of $[ 0, 128 - F_n )$, such that, for all the timesteps, the range of bins $[ F_s, F_s + F_n )$ is masked by setting the power value in the spectrogram to 0. Afterwards, we resize the spectrogram height to a value randomly chosen from the interval $[224, 320]$, and finally select a random $224 \times 224$ crop. 

During inference, we do not perform time and frequency masking, we simply resize the height of the spectrogram to $224$ and select a $224 \times 224$ central crop for each frame.

We use the obtained spectrogram repeated 3 times to construct a 3-channel input for the Swin-T backbone. Despite the simple setup, our audio-specific model performs on par with more sophisticated state-of-the-art audio models \cite{stergiou2022play} on Epic-Kitchens.

\subsection{Object Detections (OBJ)}
When pre-processing the Object Detections (on Something-Something and Something-Else) we closely follow the setup of \textbf{Chapter~\ref{ch:bmvc2021}}. We represent each video frame with only its object detections---bounding boxes \& object categories. We use the object detections released from Herzig~\etal~\cite{herzig2022object} for Something-Something and Materzynska~\etal~\cite{materzynska2020something} for Something-Else, which had been obtained using a Faster R-CNN \cite{ren2015faster}, trained as per the setting of \cite{shan2020understanding}. We use the \blackgls{stlt} (Spatial-Temporal Layout Transformer) model to encode the object detections, while following the settings and the implementation of \textbf{Chapter~\ref{ch:bmvc2021}}.
% In the \blackgls{stlt} model, one Transformer model \cite{vaswani2017attention} encodes the spatial relations between the objects in each frame independently, while another Transformer encodes the temporal relations given the embedding of each frame (output of the Spatial-Transformer).

\section{Details on Action Recognition Models Trained on Multimodal Data}\label{iccv2023:appendix:omnivore}
Multiple works explore a similar setting, i.e., using multiple modalities for training while performing inference using only RGB frames. Some of the most prominent works are ModDrop \cite{neverova2015moddrop}, DMCL \cite{garcia2018modality, garcia2019dmcl}, and Omnivore \cite{girdhar2022omnivore}.

\textbf{ModDrop.} Neverova~\etal~\cite{neverova2015moddrop} propose a method where a multimodal model is made robust to missing modalities during inference by randomly dropping out modalities during training. Namely, the model is trained to observe all modalities, a partial set of modalities, or only a single modality during training. This makes the model recognize cues, generally multimodal, from RGB data, and is therefore superior to an RGB model.

\textbf{DMCL.} Garcia~\etal~\cite{garcia2018modality, garcia2019dmcl} propose a four-step multimodal distillation framework which is tested on non-egocentric data. They train a model on multimodal inputs, where for each training video-action sample, the teacher network is established as the model that exhibits the lowest cross-entropy w.r.t. ground truth action, and the remaining models are the students. Then, the student models are trained on the soft teacher labels. On the other hand, our method is simple---standard knowledge distillation---and flexible---other models can easily be added to the ensemble, and the student model can be retrained while keeping the existing models fixed.

\textbf{Omnivore.} \cite{girdhar2022omnivore} To the best of our knowledge, Omnivore is the latest and best-performing method that uses multimodal data during training, while using only unimodal data during inference. Compared to multimodal distillation, Omnivore can perform inference using a single set of weights across all different modalities it was trained on. In particular, Girdhar~\etal~\cite{girdhar2022omnivore} use multimodal data during pre-training, while for the downstream task, the model is directly fine-tuned on the RGB frames. The resulting model---pre-trained on omnivorous data---is superior. In our work, to establish an Omnivore baseline parallel to multimodal distillation, we perform training on the multimodal data and the downstream task features.

To train a single model (single set of weights) using multimodal data, Girdhar~\etal~\cite{girdhar2022omnivore} propose two strategies to sample the batches: (i) Batches contain data of mixed modalities (heterogenous batches), or (ii) each batch is unimodal (homogenous) with a randomly chosen modality. In our work, we found that (i) yields a model with performance similar to simply training the model on RGB frames, and therefore, we opted for (ii).

\section{Implementation Details}\label{iccv2023:appendix:experimental-setup}
We train all models for 60 epochs using AdamW \cite{loshchilov2017decoupled}, with a peak learning rate of $1e-4$, linearly increased for the first 5\% of the training and decreased to 0.0 by the end of the specified 60 epochs. We use weight decay with a regularization coefficient of $5e-2$, and clip the gradients when their norm exceeds 5.0. For Epic-Kitchens, we sample 32 frames with a fixed stride of 2, and for Something-Something and Something-Else we evenly sample 16 frames to cover the whole video. We use a single spatial and temporal crop, unless stated otherwise. During training, we chose a random start frame, while during inference, we select the start frame such that the sequence covers the central portion of the video. If we use multiple temporal crops as test-time augmentation, we choose the start frames such that the video is covered uniformly. During training we apply standard data augmentations---random spatial video crops, color jittering, and horizontal flips (for Epic-Kitchens only). The temperature parameter $\tau$ is fixed to 10.0 for both the student and the teacher during multimodal knowledge distillation. In \S\ref{iccv2023:sec:weighting} we ablate the impact of the loss balancing term $\lambda$ and the Ensemble Teacher Weighting temperature term $\gamma$\footnote{As the datasets' test sets either do not exist \cite{materzynska2020something}, or have restricted access, we report results using the model after the final training epoch.}.

During training we follow the consistent teaching paradigm \cite{beyer2022knowledge} where the student and teacher strictly receive the same views of the data---we ensure spatial and temporal consistency, i.e., the models receive the same frame indices, same random crops, and horizontal flips.
